# Supplementary material for: Few-Photon Scattering in Dispersive Waveguides with Multiple Qubits
Source: arXiv:1603.02920 ancillary file (2016-05-21)
Supplement: Supplementary file 1 [file code_documentation.pdf]

## main.m Driver Program Used in the Generation of Figures

This file is the main driver of the Krylov subspace based time evolution code. The code is capable of simulating an arbitrary number of qubits and it uses the occupation number basis states so as to decrease the computational requirements. Computations are split into multiple files and the flowchart for the code is as sketched below. The filenames for each section are represented in parantheses with a `monospaced` font. There are three figures in the paper. All of them are created using the flowchart below, with changes in the setup, and what is being measured.

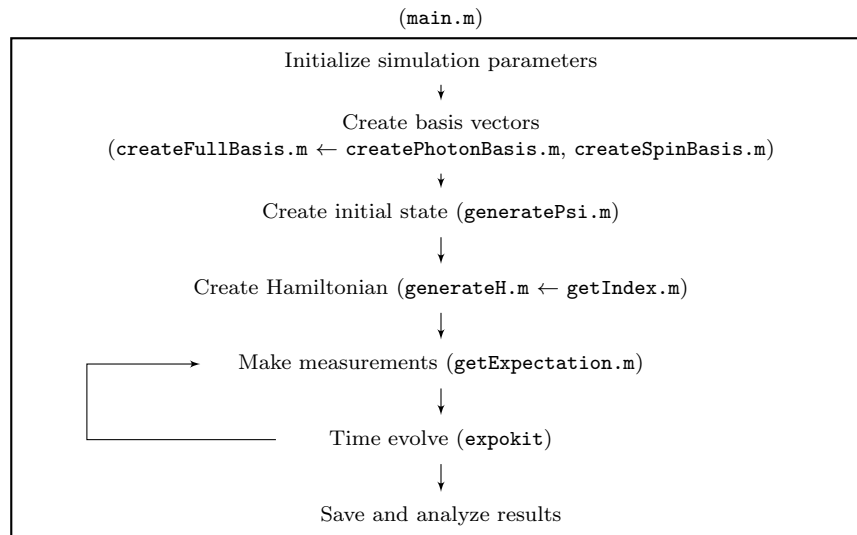

## Contents

- Fig 1a: One-Atom Multiple-Photon Scattering
- Fig 1b: Two-Atom One-Photon Scattering
- Fig 2: Time Evolution of Doubly Excited Two-Atom System
- Fig 3: Analysis of the Fidelity of a Pauli (-Z) Gate

### Fig 1a: One-Atom Multiple-Photon Scattering

```
clear all
close all
clc
```

For time evolution we will use the `expokit` matlab files.<sup>1</sup>

```
if isempty(which('expv'))
    addpath('./expokit/matlab');
end
```

```
% number of photons, m, go from 1 to 4
for m=1:4
```

```
    % Do not run the simulation if the relevant data file exists
    if exist(sprintf('./results/fig1/nbList_m%d.tsv',m),'file')
        continue;
    end

    tic
```

These global variables are used to communicate with different functions within the code. The lack of pointers in Matlab led to this design choice.

<sup>1</sup>See <http://www.maths.uq.edu.au/expokit/> for the source code and <http://dl.acm.org/citation.cfm?id=285868> for the paper that explains the technique.

```

global indexList; % holds a variety of indices, see createFullBasis.m
global bosonBasis; % holds the bosonic part of the basis
global spinBasis; % holds the spin part of the basis
global psiInitial; % the initial wave function
global psi; % wave function at the next time instant

% Simulation parameters
J = 1; % hopping parameter
V = J; % coupling parameter
Omega = sqrt(2)*J; % qubit energy separation
L = 99; % lattice length
x0 = 50; % qubit position

% Initial state consists of m photons with the qubit in the down state
% There is only a single sector in the initial state
% The initial state is composed of a Gaussian pulse of m photons
% freephoton_handle function is created with k0, xc, s
n = 1; % number of qubits
k0 = 3*pi/4; % center k-vector of the Gaussian
xc = 26; % center of the Gaussian at t=0, should be away from boundaries
s = 5; % Spatial width of the Gaussian

freephoton_handle = @(x) 1/(pi*s^2)^(0.25) * ...
    exp(-(x-xc).^2./(2*s.^2)) .* exp(1i*k0*x);

initialStateParams= struct('weights', {1}, ...
    'qubitStates',{[0]}, ...
    'photonStates', {repmat({freephoton_handle},1,m)});

% Create basis
createFullBasis(m,n,L);
disp('Basis creation done.')

% Create initial state
generatePsi(initialStateParams);
disp('Initial state creation done.')

% Create Hamiltonian
H = generateH(J,Omega,V,x0);
disp('Hamiltonian creation done.')

% Time evolve and make measurements
delT = 2; % time increment used
tlist = 0:delT:50; % time list variable
nbList = zeros(size(tlist)); % stores qubit excitation, see getExpectation.m
nxList = zeros(length(tlist),L); % stores photonic expectation
RList = zeros(size(tlist)); % stores reflection coefficients
TList = zeros(size(tlist)); % stores transmission coefficients

psi = psiInitial;

for ii=1:length(tlist)
    t = tlist(ii);
    % make measurements
    [nx,nb,R,T] = getExpectation(x0);
    nxList(ii,:) = nx;
    nbList(ii) = nb;
    RList(ii) = R;
    TList(ii) = T;
    fprintf('t=%d\n',t)
    % time evolve

```

```

        psiInitial = psi;
        psi = expv(delT,-1i*H,psiInitial);
    end

    totalTime=toc;
    fprintf('Fig 1a: %d photon calculation took %06.0f sec.',m,totalTime);

    % Export nbList as tab separated list for pgfplot
    dum=[tlist;nbList]';
    filename = sprintf('./results/fig1/nbList_m%d.tsv',m);
    dlmwrite(filename, dum, 'delimiter', '\t', 'precision', '%0.6e');

end

% Comparison of data with published results
plotColor={'k.' 'b.' 'r.' 'g.'};

% Put the cropped figure as a background on the axis
figure;
hold on
x = imread('./doc/figs/Longo2010_fig2.png');
image([0 50],[0.4 0],x);
title('Comparison to Longo2010 Fig 2','interpreter','latex');

% Superpose the simulation data on the plot
for ii=1:m
    dum=load(sprintf('./results/fig1/nbList_m%d.tsv',ii));
    plot(dum(:,1),dum(:,2),plotColor{ii},'MarkerSize',20)
end
xlim([0 50]); ylim([0 0.4]);
ax = gca;
outerpos = get(ax,'OuterPosition');
ti = get(ax,'TightInset');
left = outerpos(1) + ti(1);
bottom = outerpos(2) + ti(2);
ax_width = outerpos(3) - ti(1) - ti(3);
ax_height = outerpos(4) - ti(2) - ti(4);
set(ax,'Position', [left bottom ax_width ax_height]);
fig = gcf;
set(fig,'PaperPositionMode','auto');
fig_pos = get(fig,'PaperPosition');
set(fig,'PaperSize',[fig_pos(3) fig_pos(4)]);
print(gcf,'./results/fig1/fig1a.pdf','-dpdf');

```

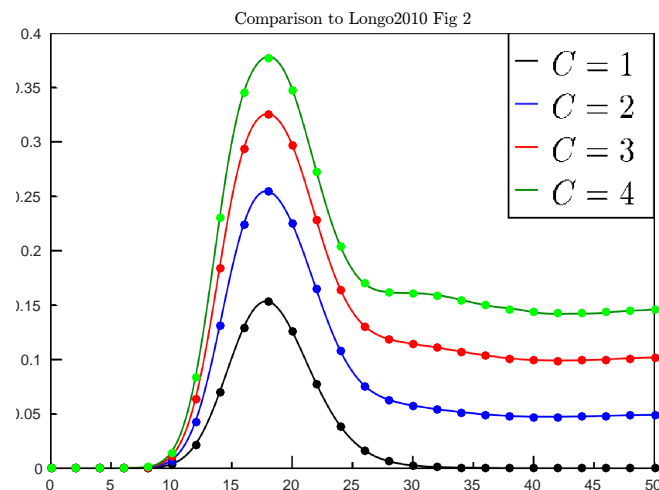

As is shown above, there is perfect agreement between the results from the Longo2010 paper (solid lines) and those from this code's results (filled circles). Whereas in Longo2010 the calculations for 3 and 4 photons were

done using the DMRG technique, here we are able to do the same set of simulations via direct diagonalization. Simulations took 1, 5, 162 and 7102 seconds for 1 to 4 photons, respectively. 4 photon calculations require a 64 bit machine with enough RAM.

### Fig 1b: Two-Atom One-Photon Scattering

We will calculate the reflection and transmission coefficients of the photon scattering from a two-qubit system and compare the results with analytical formulas. First, we provide some details to give more information on the derivations leading to Eq. (3) in the paper.

The system of interest is as shown below. Qubits are numbered from left to right. Left qubit has index 1, right qubit has index 2.

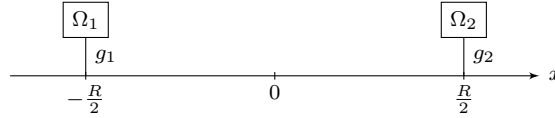

The Hamiltonian for the system is derived using the dipole and rotating wave approximations as  $H = H_0 + V$  with  $(\hbar = 1)$

$$H_0 = \frac{\Omega_1}{2}\sigma_{z_1} + \frac{\Omega_2}{2}\sigma_{z_2} + \int_{-\pi}^{\pi} dk \omega_k a_k^\dagger a_k,$$

$$V = g_1 \int_{-\pi}^{\pi} dk \sigma_1^+ e^{-ikR/2} a_k + g_2 \int_{-\pi}^{\pi} dk \sigma_2^+ e^{+ikR/2} a_k + \text{h.c.} \quad (1)$$

where h.c. stands for hermitian conjugate,  $\sigma_{z_i}, \sigma_i^\pm$  are the Pauli matrices for qubit  $i$ ,  $a_k$  is the annihilation operator for a photon with wave-vector  $k$ ,  $\omega_k = -2J \cos k$  is the tight-binding dispersion relation of the waveguide,  $g_i$  are the coupling constants between the qubits and the waveguide modes.

We will label the orthogonal modes in the single excitation sector as  $|k\downarrow_1\downarrow_2\rangle$ ,  $|\uparrow_1\downarrow_2\rangle$  and  $|\downarrow_1\uparrow_2\rangle$  where the arrow subscripts are qubit indices. To make the notation more concise, we will drop the qubit indices, and bras and kets will have the qubits ordered from left to right according to their index. We will be making use of the resolvents for  $H$  and  $H_0$  defined as  $G(z) = (z - H)^{-1}$  and  $G_0(z) = (z - H_0)^{-1}$  while deriving the scattering matrix of the system. The particular matrix element we are interested in is

$$\langle p\downarrow\downarrow|S|k\downarrow\downarrow\rangle = \langle p\downarrow\downarrow|k\downarrow\downarrow\rangle - 2\pi i \delta(\omega_p - \omega_k) \lim_{\eta \rightarrow 0^+} \langle p\downarrow\downarrow|T(\omega_p - \frac{\Omega_1 + \Omega_2}{2} + i\eta)|k\downarrow\downarrow\rangle. \quad (2)$$

The  $T$ -matrix elements are related to the matrix elements of the resolvent through the relationship

$$G(z) = G_0(z) + G_0(z)T(z)G_0(z).$$

Therefore, we need to find  $\langle p\downarrow\downarrow|G|k\downarrow\downarrow\rangle$  to get the  $S$ -matrix element we are after. We will also be interested in the remainder eight matrix elements  $\langle p\downarrow\downarrow|G|\uparrow\downarrow\rangle$ ,  $\langle p\downarrow\downarrow|G|\downarrow\uparrow\rangle$ ,  $\langle \uparrow\downarrow|G|k\downarrow\downarrow\rangle$ ,  $\langle \uparrow\downarrow|G|\uparrow\downarrow\rangle$ ,  $\langle \uparrow\downarrow|G|\downarrow\uparrow\rangle$ ,  $\langle \downarrow\uparrow|G|k\downarrow\downarrow\rangle$ ,  $\langle \downarrow\uparrow|G|\uparrow\downarrow\rangle$ ,  $\langle \downarrow\uparrow|G|\downarrow\uparrow\rangle$  as well. We will use the Lippmann-Schwinger equation for the resolvent

$$G = G_0 + G_0VG \quad (3)$$

$$= G_0 + GVG_0, \quad (4)$$

and the identity operator for two-qubits in the single excitation sector

$$\mathbf{1} = |\uparrow\downarrow\rangle\langle\uparrow\downarrow| + |\downarrow\uparrow\rangle\langle\downarrow\uparrow| + \int_{-\pi}^{\pi} dk |k\downarrow\downarrow\rangle\langle k\downarrow\downarrow|, \quad (5)$$

as well as the orthogonality of the basis vectors  $\langle p\downarrow\downarrow|k\downarrow\downarrow\rangle = \delta(p - k)$ ,  $\langle \uparrow\downarrow|\downarrow\uparrow\rangle = \langle \downarrow\uparrow|\uparrow\downarrow\rangle = 1$ . Lastly, note that  $|k\downarrow\downarrow\rangle$ ,  $|\uparrow\downarrow\rangle$  and  $|\downarrow\uparrow\rangle$  are eigenstates of  $H_0$  hence we get

$$G_0(z)|k\downarrow\downarrow\rangle = \frac{1}{z - \omega_k + \frac{\Omega_1 + \Omega_2}{2}}|k\downarrow\downarrow\rangle,$$

$$G_0(z)|\uparrow\downarrow\rangle = \frac{1}{z - \frac{\Omega_1}{2} + \frac{\Omega_2}{2}}|\uparrow\downarrow\rangle,$$

$$G_0(z)|\downarrow\uparrow\rangle = \frac{1}{z + \frac{\Omega_1}{2} - \frac{\Omega_2}{2}}|\downarrow\uparrow\rangle.$$

Let us define nine functions corresponding to the nine matrix elements as follows

$$\begin{aligned} G_1(z) &= \langle \uparrow\downarrow | G | \uparrow\downarrow \rangle & G_2(z) &= \langle \uparrow\downarrow | G | \downarrow\uparrow \rangle & G_3(z; k) &= \langle \uparrow\downarrow | G | k\downarrow\downarrow \rangle \\ G_4(z) &= \langle \downarrow\uparrow | G | \uparrow\downarrow \rangle & G_5(z) &= \langle \downarrow\uparrow | G | \downarrow\uparrow \rangle & G_6(z; k) &= \langle \downarrow\uparrow | G | k\downarrow\downarrow \rangle \\ G_7(z; p) &= \langle k\downarrow\downarrow | G | \uparrow\downarrow \rangle & G_8(z; p) &= \langle k\downarrow\downarrow | G | \downarrow\uparrow \rangle & G_9(z; p, k) &= \langle k\downarrow\downarrow | G | k\downarrow\downarrow \rangle. \end{aligned}$$

Calculation of the one-photon scattering matrix element requires the knowledge of  $G_9(z; p, k)$ . We will now solve for  $G_9$ . Through the use of (3), (5) and (1) we get

$$\begin{aligned} G_9(z; p, k) &= \langle p\downarrow\downarrow | G | k\downarrow\downarrow \rangle = \langle p\downarrow\downarrow | G_0 + G_0 V \mathbf{1} G | k\downarrow\downarrow \rangle \\ &= \frac{\delta(p-k)}{z - \omega_k + \frac{\Omega_1 + \Omega_2}{2}} + \frac{\langle p\downarrow\downarrow | V \mathbf{1} G | k\downarrow\downarrow \rangle}{z - \omega_p + \frac{\Omega_1 + \Omega_2}{2}} \\ &= \frac{\delta(p-k)}{z - \omega_k + \frac{\Omega_1 + \Omega_2}{2}} + \frac{\langle p\downarrow\downarrow | V | \uparrow\downarrow \rangle \langle \uparrow\downarrow | G | k\downarrow\downarrow \rangle + \langle p\downarrow\downarrow | V | \downarrow\uparrow \rangle \langle \downarrow\uparrow | G | k\downarrow\downarrow \rangle}{z - \omega_p + \frac{\Omega_1 + \Omega_2}{2}} \\ &= \frac{\delta(p-k)}{z - \omega_k + \frac{\Omega_1 + \Omega_2}{2}} + \frac{g_1 e^{ip\frac{R}{2}} G_3(z) + g_2 e^{-ip\frac{R}{2}} G_6(z)}{z - \omega_p + \frac{\Omega_1 + \Omega_2}{2}}. \end{aligned}$$

Similarly, for  $G_3$  and  $G_6$  via the use of (4) we get

$$\begin{aligned} G_3(z; k) &= \frac{g_1 e^{-ik\frac{R}{2}} G_1(z) + g_2 e^{+ik\frac{R}{2}} G_2(z)}{z - \omega_k + \frac{\Omega_1 + \Omega_2}{2}} \\ G_6(z; k) &= \frac{g_1 e^{-ik\frac{R}{2}} G_4(z) + g_2 e^{+ik\frac{R}{2}} G_5(z)}{z - \omega_k + \frac{\Omega_1 + \Omega_2}{2}}. \end{aligned} \quad (6)$$

We again apply (4) to  $G_1$  and  $G_2$  to get

$$G_1(z) = \frac{1 + \int_{-\pi}^{\pi} dk G_3(z; k) g_1 e^{+ik\frac{R}{2}}}{z - \frac{\Omega_1}{2} + \frac{\Omega_2}{2}} \quad (7)$$

$$G_2(z) = \frac{\int_{-\pi}^{\pi} dk G_3(z; k) g_2 e^{-ik\frac{R}{2}}}{z + \frac{\Omega_1}{2} - \frac{\Omega_2}{2}}. \quad (8)$$

We can now solve for  $G_1$ ,  $G_2$  and  $G_3$  by using (6), (7) and (8). The result is

$$\begin{aligned} G_1(z) &= \frac{z' - \Omega_2 - g_2^2 I(z'; 0)}{D} \\ G_2(z) &= \frac{g_1 g_2 I(z'; -R)}{D}. \end{aligned}$$

Here, the denominator function is given by

$$D = [z' - \Omega_1 - g_1^2 I(z'; 0)][z' - \Omega_2 - g_2^2 I(z'; 0)] - g_1^2 g_2^2 I(z'; R) I(z'; -R),$$

and  $z' = z + \frac{\Omega_1 + \Omega_2}{2}$ . Also, the  $I$  function is defined through the integral

$$I(z; x) = \lim_{\eta \rightarrow 0^+} \int_{-\pi}^{\pi} dk \frac{e^{ikx}}{z - \omega_k + i\eta}$$

for which when  $\omega_k = -2J \cos k$  and with  $z \in (-2J, 2J)$  we use the residue theorem to get

$$I(z; x) = \frac{(-2\pi i) e^{ik_* |x|}}{\sqrt{4J^2 - z^2}} = \frac{(-2\pi i) e^{ik_* |x|}}{2J |\sin k_*|},$$

where  $k_* = \arccos \frac{-z}{2J}$ . With a very similar set of calculations we arrive at

$$\begin{aligned} G_4(z) &= \frac{g_1 g_2 I(z'; R)}{D} \\ G_5(z) &= \frac{z' - \Omega_1 - g_1^2 I(z'; 0)}{D}. \end{aligned}$$

We now have all the matrix elements of  $G(z)$  to calculate the  $S$ -matrix in (2). Substitution and some algebra results in the equations in the main text.

```

clear all

if ~exist('./results/fig1/RTdata.tsv','file') || ...
    ~exist('./results/fig1/RTIntdata.tsv','file') || ...
    ~exist('./results/fig1/RTBaredata.tsv','file')

    global indexList; global bosonBasis; global spinBasis;
    global psiInitial; global psi;

    % Simulation parameters
    J = 1; % hopping parameter
    V1 = 0.4; % coupling parameter for qubit 1
    V2 = 0.2; % coupling parameter for qubit 2
    Omega1 = 0.4; % qubit 1 energy separation
    Omega2 = 0.8; % qubit 2 energy separation
    L = 399; % lattice length
    Rsep = 5 ; % separation between qubits
    x01 = ceil(L/2); % qubit 1 position
    x02 = ceil(L/2)+Rsep; % qubit 2 position
    delT = 1; % delta time step

    % Initial state consists of m photons with the qubits in the down state
    % There is only a single sector in the initial state
    m = 1; % number of excitations
    n = 2; % number of qubits
    mink = pi/6; % minimum k value for Gaussian pulse center
    maxk = 5*pi/6; % maximum k value for Gaussian pulse center
    omega1k = acos(-Omega1/(2*J)); % resonant k value for Omega1
    omega2k = acos(-Omega2/(2*J)); % resonant k value for Omega2
    deltak1 = pi/100; % rough parameter sweep discretization for pulse center
    deltak2 = pi/500; % fine parameter sweep discretization for pulse center
    klist = [(mink:deltak1:omega1k*0.95) (omega1k*0.95:deltak2:1.05*omega2k) ...
        (1.05*omega2k:deltak1:maxk)']; % discretized k values
    xc = 41; % pulse center
    s = 20; % pulse width
    NT = 50; % number of time sim points
    % These variables hold the sim results
    RStorage = zeros(length(klist),1); % reflection (R) coefficients
    TStorage = zeros(length(klist),1); % transmission (T) coefficients
    % These functions are used in numerical integration
    % They are from Eq. (3) in the paper
    r1 = @(k) -V1^2 ./ ((2*1i*J*abs(sin(k)).*(Omega1+2*J*cos(k)))+V1^2);
    r2 = @(k) -V2^2 ./ ((2*1i*J*abs(sin(k)).*(Omega2+2*J*cos(k)))+V2^2);
    t1 = @(k) 1+r1(k);
    t2 = @(k) 1+r2(k);
    r_func = @(k) (2.*r1(k).*r2(k).*exp(1i*k*Rsep)+r1(k).*exp(-1i*k*Rsep)+ ...
        +r2(k).*exp(1i*k*Rsep))./(1-r1(k).*r2(k).*exp(2*1i*k*Rsep));
    t_func = @(k) (t1(k).*t2(k))./(1-r1(k).*r2(k).*exp(2*1i*k*Rsep));
    RIntStorage = zeros(length(klist),1); % R integral results
    TIntStorage = zeros(length(klist),1); % T integral results
    RBareStorage = zeros(length(klist),1); % non-integrated R data
    TBareStorage = zeros(length(klist),1); % non-integrated T data

    for kk = 1:length(klist)

        k0 = klist(kk);

        % Gaussian pulse in spatial coordinates
        freephoton_x = @(x) 1/(pi*s^2)^(0.25) * ...
            exp(-(x-xc).^2./(2*s.^2)) .* exp(1i*k0*x);

```

```

% Gaussian pulse in k-space coordinates
freephoton_k = @(k) 1/(pi*1/s^2)^(0.25) * ...
    exp(-(k-k0).^2./(2*1/s.^2)) .* exp(-1i*(k-k0)*xc);

initialStateParams= struct('weights', {1}, ...
    'qubitStates',{[0 0]}, ...
    'photonStates', {repmat({freephoton_x},1,m)});

createFullBasis(m,n,L);
generatePsi(initialStateParams);
H = generateH(J,[Omega1 Omega2],[V1 V2],[x01 x02]);

% Due to dispersion, different k packets travel at different speeds
% Sine term gives the group velocity at center k value
% We run the simulations until the packets travel the same total
% distance
tmax = ceil((L/2 + L/2-xc)/(2*sin(klist(kk))));
delT = tmax/(NT-1);
tlist = linspace(0,tmax,NT);

nsList = zeros(length(tlist),n); % expectation value for the two qubits
nxList = zeros(length(tlist),L); % expectation value for photons
RList = zeros(size(tlist)); % reflection coefficient
TList = zeros(size(tlist)); % transmission coefficient

psi = psiInitial;

for ii=1:length(tlist)
    t = tlist(ii);
    [nx,ns,R,T] = getExpectation([x01 x02]);
    nxList(ii,:) = nx;
    nsList(ii,:) = ns;
    RList(ii) = R;
    TList(ii) = T;
    psiInitial = psi;
    psi = expv(delT,-1i*H,psiInitial);
end

RStorage(kk) = RList(end);
TStorage(kk) = TList(end);
RIntStorage(kk) = integral(@(k) abs(r_func(k).*freephoton_k(k)).^2,...
    k0-pi,k0+pi,'AbsTol',1e-12,'RelTol',1e-8);
TIntStorage(kk) = integral(@(k) abs(t_func(k).*freephoton_k(k)).^2,...
    k0-pi,k0+pi,'AbsTol',1e-12,'RelTol',1e-8);
RBareStorage(kk) = abs(r_func(k0)).^2;
TBareStorage(kk) = abs(t_func(k0)).^2;
fprintf('k %d of %d \n',kk,length(klist))
end

% Export R,T as tab separated list for pgfplot
dum=[klist,RStorage,TStorage];
filename = './results/fig1/RTdata.tsv';
dlmwrite(filename, dum, 'delimiter', '\t', 'precision', '%0.6e');

dum=[klist,RIntStorage,TIntStorage];
filename = './results/fig1/RTIntdata.tsv';
dlmwrite(filename, dum, 'delimiter', '\t', 'precision', '%0.6e');

dum=[klist,RBareStorage,TBareStorage];
filename = './results/fig1/RTBaredata.tsv';
dlmwrite(filename, dum, 'delimiter', '\t', 'precision', '%0.6e');

```

```

end

% Plot the results
figure
dum = load('./results/fig1/RTdata.tsv');
dum2 = load('./results/fig1/RTIntdata.tsv');
dum3 = load('./results/fig1/RTBaredata.tsv');
plot(dum(:,1),dum(:,2),'b');
hold on;
plot(dum2(:,1),dum2(:,2),'b. ');
plot(dum3(:,1),dum3(:,2),'Color',[0.7 0.7 0.7]);
title('Single Photon Reflection from Two-Qubits','interpreter','latex');
xlabel('k_0');
ax = gca;
outerpos = get(ax,'OuterPosition');
ti = get(ax,'TightInset');
left = outerpos(1) + ti(1);
bottom = outerpos(2) + ti(2);
ax_width = outerpos(3) - ti(1) - ti(3);
ax_height = outerpos(4) - ti(2) - ti(4);
set(ax,'Position',[left bottom ax_width ax_height]);
fig = gcf;
set(fig,'PaperPositionMode','auto');
fig_pos = get(fig,'PaperPosition');
set(fig,'PaperSize',[fig_pos(3) fig_pos(4)]);
print(gcf,'./results/fig1/fig1b.pdf','-dpdf');

```

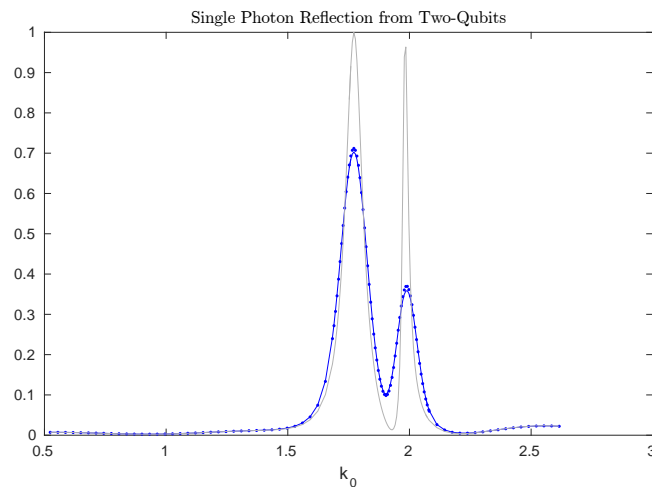

As can be seen, the integration of the analytical formulas (dots) and the results of numerical simulations (blue curve) agree very well with each other. The gray curve is the plot of the analytical reflection coefficient  $|r_k|^2$ . Gaussian integration with a finite width results in the reduction of the peak values of reflection and smoothens the graph.

## Fig 2: Time Evolution of Doubly Excited Two-Atom System

Now, we will prepare an initial state of two excited atoms and compare their time evolution as a function of time. The aim is to observe the formation of a bound state in continuum.

```

clear all

if ~exist('./results/fig2/RT_timedata.tsv','file') || ...
    ~exist('./results/fig2/ns_timedata.tsv','file') || ...
    ~exist('./results/fig2/nx_timedata.tsv','file')

    global indexList; global bosonBasis; global spinBasis;

```



```

global psiInitial; global psi;

% Simulation parameters
J = 1; % hopping parameter
V = 0.5; % coupling parameter
L = 299; % lattice length
Rsep = 5 ; % separation between qubits
x01 = ceil(L/2); % qubit 1 position
x02 = ceil(L/2)+Rsep; % qubit 2 position
delT = 0.5; % delta time step
Tmax = 70; % maximum time
order = 1; % solution order for the bound state
kRes = (2*order-1)*pi/Rsep; % resonant k-vector for even mode
%kRes = (2*order-0)*pi/Rsep; % resonant k-vector for odd mode
Omega = -2*J*cos(kRes); % resonant energy = Omega set equal

% Initial state consists of both qubits in the up state
m = 2; % number of excitations
n = 2; % number of qubits

initialStateParams= struct('weights', {1}, ...
    'qubitStates',{[1 1]}, ...
    'photonStates', {{}});

createFullBasis(m,n,L); % Create basis
generatePsi(initialStateParams); % Create initial state
H = generateH(J,[Omega Omega],[V V],[x01 x02]); % Create Hamiltonian

% Time evolve and make measurements
tlist = (0:delT:Tmax)'; % time variable values
nsList = zeros(length(tlist),n); % expectation value for the two qubits
nxList = zeros(length(tlist),L); % expectation value for photons
RList = zeros(size(tlist)); % reflection coefficient
TList = zeros(size(tlist)); % transmission coefficient

psi = psiInitial;

for ii=1:length(tlist)
    t = tlist(ii);
    [nx,ns,R,T] = getExpectation([x01 x02]);
    nxList(ii,:) = nx;
    % We output the probability of observing doubly excited state and
    % the probability of observing the first qubit in its excited level
    nsList(ii,:) = [abs(psi(end)).^2 ns(1)];
    RList(ii) = R;
    TList(ii) = T;
    fprintf('Fig 2: t=%d of %d\n',ii,length(tlist));
    psiInitial = psi;
    psi = expv(delT,-1i*H,psiInitial);
end

% Export R,T,nx,ns as tab separated list for pgfplot
dum=[tlist,RList,TList];
filename = './results/fig2/RT_timedata.tsv';
dlmwrite(filename, dum, 'delimiter', '\t', 'precision', '%0.6e');

dum=[tlist,nsList];
filename = './results/fig2/ns_timedata.tsv';
dlmwrite(filename, dum, 'delimiter', '\t', 'precision', '%0.6e');

filename = './results/fig2/nx_timedata.tsv';

```

```

    dlmwrite(filename, nxList, 'delimiter', '\t', 'precision', '%0.6e');

end % if exists(...) end

% Plot the results
dum = load('./results/fig2/RT_timedata.tsv');
dum2 = load('./results/fig2/ns_timedata.tsv');
dum3 = load('./results/fig2/nx_timedata.tsv');
figure
subplot(2,1,1) % qubit excitations
plot(dum2(:,1),dum2(:,2),'k',dum2(:,1),dum2(:,3),'r')
xlabel('Time');
ylabel('Qubit Excitation');
legend('Doubly Excited', 'Qubit 1');
title('Time Evolution of Two Excited Atoms','interpreter','latex');
subplot(2,1,2) % photon excitations
%imagesc(log10(dum3+1e-5));axis xy
imagesc(1:size(dum3,2),dum(:,1),dum3);axis xy
xlabel('Space');
ylabel('Time');
title('Photon Number Expectation','interpreter','latex');
colorbar

% Output the plot as a pdf file
ax = gca;
outerpos = get(ax,'OuterPosition');
ti = get(ax,'TightInset');
left = outerpos(1) + ti(1);
bottom = outerpos(2) + ti(2);
ax_width = outerpos(3) - ti(1) - ti(3);
ax_height = outerpos(4) - ti(2) - ti(4);
set(ax,'Position', [left bottom ax_width ax_height]);
fig = gcf;
set(fig,'PaperPositionMode','auto');
fig_pos = get(fig,'PaperPosition');
set(fig,'PaperSize',[fig_pos(3) fig_pos(4)]);
print(gcf,'./results/fig2/twoAtom_time.pdf','-dpdf');

figure;
set(gcf,'Visible','off');
imagesc(dum3,[0 0.1]); axis off;axis xy;axis square;
colormap jet;
set(gcf,'PaperUnits','inches','PaperPosition',[0 0 3 3],'PaperSize',[3 3]);
set(gcf,'RendererMode','manual','Renderer','opengl');
set(gcf,'PaperPositionMode','manual');
set(gcf,'Units','inches','Position',[0 0 3 3]);
set(gca,'PlotBoxAspectRatioMode','manual');
set(gca,'PlotBoxAspectRatio',[1 1 1]);
set(gca,'Units','inches','Position',[0 0 3 3]);
set(gcf,'Position',[5 5 3 3]);
set(gcf,'Visible','on'); set(gcf,'Position',[5 5 3 3]);
set(gcf,'PaperPositionMode','auto');
print(gcf,'./results/fig2/photonPlot.png','-dpng','-r600','-opengl');

```

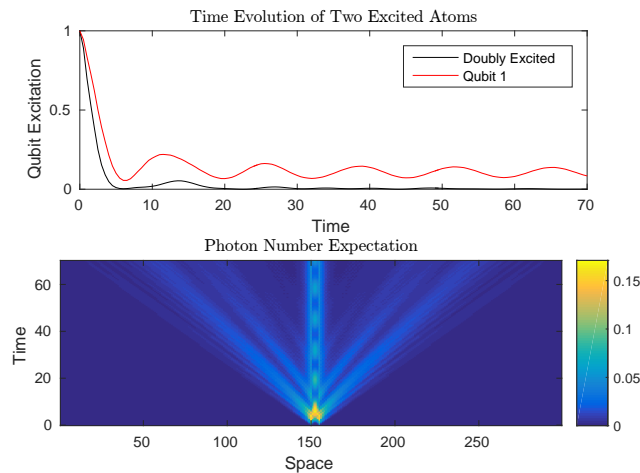

The results above show that when the separation between the qubits is at the resonant length, then, we can excite the bound state in continuum from an initially doubly excited qubit state.

### Fig 3: Analysis of the Fidelity of a Pauli (-Z) Gate

In this part, we will use the bound states in continuum to analyze the fidelity of a quantum gate formed by multiple quenches to the Hamiltonian.

```
clear all

global indexList; global bosonBasis; global spinBasis;
global psiInitial; global psi;

% Simulation parameters
% Note that these parameters are modified by hand to obtain the 4 curves
% Simply run the code with varied parameter sets, i.e. change V, Rsep,
% order variables below
J = 1; % hopping parameter
V = 0.5; % coupling parameter
L = 399; % lattice length
Rsep = 7; % separation between qubits
x01 = ceil(L/2)-Rsep; % qubit 1 position
x02 = ceil(L/2); % qubit 2 position
x03 = ceil(L/2)+Rsep; % qubit 3 position
x04 = ceil(L/2)+2*Rsep; % qubit 4 position
delT = 0.1; % delta time step
Tmax = 150; % maximum time
Tpulse = 60; % pulse duration for H_C(T) quench

% Initial state consists of m photons with the qubits in the down state
% There is only a single sector in the initial state
m = 1; % number of excitations
n = 4; % number of qubits

order = 3; % order of solution
%kRes = (2*order-1)*pi/Rsep; % resonant k-vector for even mode
kRes = (2*order)*pi/Rsep; % resonant k-vector for odd mode
Omega = -2*J*cos(kRes); % resonant energy = Omega set equal
normQubit = (2)^-0.5 * (1+V^2*Rsep/(4*J^2-Omega^2))^-0.5; % from Eq. (4)
normQubit = normQubit/sqrt(2); % since at t=0 we have a superposition of 2 BIC
normPhoton = (1+(4*J^2-Omega^2)/(V^2*Rsep))^-0.5; % analytical identity
% The function below creates the photonic part of the 2 BIC, c.f. Eq. (4)
BICphoton_handle_odd = @(x) -1i*V/sqrt(4*J^2-Omega^2) * ...
    (exp(1i*kRes*abs(x-x01)) - exp(1i*kRes*abs(x-x02)) + ...
    exp(1i*kRes*abs(x-x03)) - exp(1i*kRes*abs(x-x04)))/normPhoton;
```

```

initialStateParams= struct('weights', ...
    {normQubit -normQubit normQubit -normQubit normPhoton}, ...
    'qubitStates',{[1 0 0 0],[0 1 0 0],[0 0 1 0],[0 0 0 1],[0 0 0 0]}, ...
    'photonStates', {{},{},{},{},{BICphoton_handle_odd}});

createFullBasis(m,n,L); % Create basis
generatePsi(initialStateParams); % Create initial state
H = generateH(J,[Omega Omega Omega Omega],[V V V V],[x01 x02 x03 x04]); % Create Hamiltonian

% Hdelta is to be applied for Tpulse duration of time to result in a Pauli Z gate
Hdel = generateH(J,[Omega+pi/Tpulse Omega+pi/Tpulse Omega Omega],[V V V V],[x01 x02 x03 x04]);

% Time evolve and make measurements
tlist = 0:delT:Tmax; % time variable values
nsList = zeros(length(tlist),n); % expectation value for the two qubits
nxList = zeros(length(tlist),L); % expectation value for photons
RList = zeros(size(tlist)); % reflection coefficient
TList = zeros(size(tlist)); % transmission coefficient
qubitList = zeros(n,length(tlist)); % state of qubits
psi = psiInitial;

for ii=1:length(tlist)
    % First measure
    t = tlist(ii);
    [nx,ns,R,T] = getExpectation([x01 x02]);
    nxList(ii,:) = nx;
    nsList(ii,:) = ns;
    RList(ii) = R;
    TList(ii) = T;
    if mod(ii,50)==0 fprintf('Fig 3: t=%d of %d\n',ii,length(tlist)); end;
    % indexList is ordered from lowest spin state to highest spin state
    % qubitList is ordered from leftmost qubit to rightmost qubit which is
    % actually in a reverse order compared to indexList.
    % Evaluate the following code to get a better insight
    % spinBasis(indexList(5:-1:2,5),:)
    % see also documentation of createFullBasis.m
    qubitList(:,ii) = psi(indexList(5:-1:2,1));

    % Then time evolve
    psiInitial = psi;
    if (t<10+Tpulse) && (t >= 10)
        % Application of gate operation for a limited time for a pi pulse
        psi = expv(delT,-1i*Hdel,psiInitial);
    else
        psi = expv(delT,-1i*H,psiInitial);
    end
end

% Plot the results
figure
subplot(2,2,1)
plot(real(qubitList(1,:)),imag(qubitList(1:)), 'k-'); hold on;
plot(real(qubitList(2,:)),imag(qubitList(2:)), 'b-');
plot(real(qubitList(3,:)),imag(qubitList(3:)), 'r-');
plot(real(qubitList(4,:)),imag(qubitList(4:)), 'g-');
plot(real(qubitList(1,1)),imag(qubitList(1,1)), 'ko');
plot(real(qubitList(2,1)),imag(qubitList(2,1)), 'bo');
plot(real(qubitList(3,1)),imag(qubitList(3,1)), 'ro');
plot(real(qubitList(4,1)),imag(qubitList(4,1)), 'go');
legend('\uparrow\downarrow\downarrow\downarrow\rangle',...

```

```

        '\downarrow\uparrow\downarrow\downarrow\rangle',...
        '\downarrow\downarrow\uparrow\downarrow\rangle',...
        '\downarrow\downarrow\downarrow\uparrow\rangle');
title('Evolution of qubit states on the complex plane','interpreter','latex');

subplot(2,2,2)
imagesc(1:L,tlist,log10(nxList+1e-5),[-5 -1]);axis xy
xlabel('Space');
ylabel('Time');
title('Photon Number Expectation','interpreter','latex');
line([0 399;0 399],[10 10;10+Tpulse 10+Tpulse'],'...
      'LineStyle','--','Color','r') % quench time shown with red dashed lines
hcb=colorbar;

subplot(2,2,3)
c= linspace(0,1,length(tlist));
colormap jet
% Exp terms below lead to the interaction picture
bit01_time=(qubitList(3,:)-qubitList(4,:)).*exp(-1i*Omega*tlist); %a_01 from paper
bit10_time=(qubitList(1,:)-qubitList(2,:)).*exp(-1i*Omega*tlist); %a_10 from paper
plot(real(bit01_time),imag(bit01_time),'k-','LineWidth',3)
hold on
plot(real(bit10_time),imag(bit10_time),'ro')
axis equal;
rectangle('Position',[-1,-1,2,2],...
          'Curvature',[1,1],'LineStyle',':') % unit circle shown with dots
title('Time Evolution of Logical Qubits','interpreter','latex')
xlim([-1.1 1.1]); ylim([-1.1 1.1]);

subplot(2,2,4)
% See Nielsen & Chuang "Quantum Computation and Quantum Information" p. 415
% for the fidelity between two pure states
bit00 = [0 0 0 0];
bit01 = ([0 0 1 0] - [0 0 0 1])/sqrt(2);
bit10 = ([1 0 0 0] - [0 1 0 0])/sqrt(2);
finalState = (bit01 - bit10)/sqrt(2); % ideal final state \psi_I in paper
fidelity = abs(finalState * qubitList);
plot(tlist,fidelity,'b','Linewidth',1);hold on;
line([10 10+Tpulse; 10 10+Tpulse],[0 0; max(fidelity) max(fidelity)],...
      'LineStyle','--','Color','r') % quench time shown with red dashed lines
title(sprintf('Fidelity at t=%d is %g',t(end),fidelity(end)),'interpreter','latex')
set(gcf,'Units','normalized','Position',[0.25 0.25 0.5 0.5]);

% Output the plot as a pdf file
ax = gca;
outerpos = get(ax,'OuterPosition');
ti = get(ax,'TightInset');
left = outerpos(1) + ti(1);
bottom = outerpos(2) + ti(2);
ax_width = outerpos(3) - ti(1) - ti(3);
ax_height = outerpos(4) - ti(2) - ti(4);
set(ax,'Position', [left bottom ax_width ax_height]);
fig = gcf;
set(fig,'PaperPositionMode','auto');
fig_pos = get(fig,'PaperPosition');
set(fig,'PaperSize',[fig_pos(3) fig_pos(4)]);
print(gcf,'./results/fig3/fourAtomGate.pdf','-dpdf');

% Export data for pgfplot
dum=[tlist,real(bit10_time),imag(bit10_time),...
      real(bit01_time),imag(bit01_time),fidelity];

```

```
filename = sprintf('./results/fig3/Zgate_R%02d_V%02.0f_Order%02d.tsv',Rsep,10*V,order);
dlmwrite(filename, dum, 'delimiter', '\t', 'precision', '%0.6e');
```

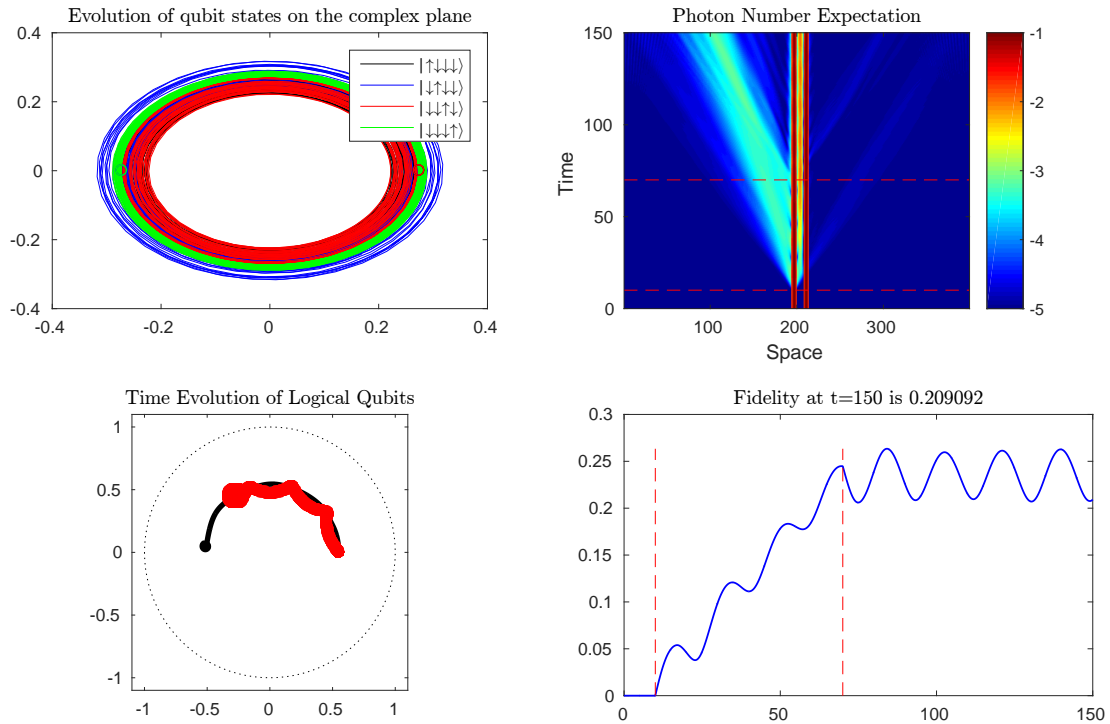

The results above show the evolution of the system under the influence of the quench. Due to the non-idealities such as photon leakage (see upper right plot) and reduced qubit weight in the BIC, the fidelity of the system is less than 1. The setup above enables one to investigate the gate dynamics as a function of system parameters. The upper left plot shows the dynamics of the relevant qubit states with circulations around the origin. When we go to the interaction picture with respect to  $H_0$  the circulations are unwound.

## createFullBasis.m Create the Full Basis Set in All Sectors

This function will use the spin and photon parts and combine them to form the full basis set. There are  $m$  total excitations in a 1D lattice of length  $L$ . The number of spins is given by  $n$ . The ordering of the basis is illustrated below for  $m \geq 3$  total excitations and three qubits. The upper part will have  $m$  photons and all spins down. Gradually the excitations will be transferred to the spin part. Below, subscript  $p$  stands for ‘photon’ and  $s$  for ‘spin.’

*Example:* Basis set for  $m$  photons,  $n = 3$  spins.

$$\begin{pmatrix} |m\rangle_p \otimes |\downarrow_1\downarrow_2\downarrow_3\rangle_s \\ |m-1\rangle_p \otimes |\downarrow_1\downarrow_2\uparrow_3\rangle_s \\ |m-1\rangle_p \otimes |\downarrow_1\uparrow_2\downarrow_3\rangle_s \\ |m-1\rangle_p \otimes |\uparrow_1\downarrow_2\downarrow_3\rangle_s \\ |m-2\rangle_p \otimes |\downarrow_1\uparrow_2\uparrow_3\rangle_s \\ |m-2\rangle_p \otimes |\uparrow_1\downarrow_2\uparrow_3\rangle_s \\ |m-2\rangle_p \otimes |\uparrow_1\uparrow_2\downarrow_3\rangle_s \\ |m-3\rangle_p \otimes |\uparrow_1\uparrow_2\uparrow_3\rangle_s \end{pmatrix} \begin{matrix} \text{sector \#1} \\ \text{sector \#2} \\ \text{sector \#3} \\ \text{sector \#4} \\ \text{sector \#5} \\ \text{sector \#6} \\ \text{sector \#7} \\ \text{sector \#8} \end{matrix}$$

```
function createFullBasis(m,n,L)
```

The outputs from the function are written to global variables as defined below.

```
global indexList;
global bosonBasis;
global spinBasis;
```

The photon part will start with  $m$  excitations, and it will go all the way down to zero excitations only if we have enough number of spins. Otherwise, there will always be some photonic excitations left,  $m_{\min}$  of them to be precise.

```
m_min = m-min(m,n);
```

The total length of the basis will be given by

$$\sum_{i=m_{\min}}^m \underbrace{\binom{L+i-1}{i}}_{\text{photon}} \underbrace{\binom{n}{m-i}}_{\text{spin}}.$$

```
totalLength = 0;
for ii=m:-1:m_min
    totalLength = totalLength + nchoosek(L+ii-1,ii)*nchoosek(n,m-ii);
end
```

We will create the spin basis first.

```
spinBasis = createSpinBasis(n);
```

Now the photon (i.e. boson) basis will be created. The boson basis will hold the basis states for  $m, m-1, \dots, m_{\min}$  number of photons in a lattice of length  $L$ .

```
bosonBasisLength = 0;
for ii=m:-1:m_min
    bosonBasisLength = bosonBasisLength + nchoosek(L+ii-1,ii);
end
bosonBasis = zeros(bosonBasisLength,L);
lastIndexBoson = 0;
for ii=m:-1:m_min
    startIndex = lastIndexBoson+1;
    endIndex = lastIndexBoson+nchoosek(L+ii-1,ii);
    bosonBasis(startIndex:endIndex,:) = createPhotonBasis(ii,L);
    lastIndexBoson = endIndex;
end
```

Associated with the spin basis and the boson basis, the `indexList` variable will hold the indices to different sectors in the basis set. Each sector refers to a different fixed collective qubit state, e.g.  $|\uparrow_1\downarrow_2\uparrow_3\rangle_s$ . The `indexList` variable will be utilized in other parts of the code, therefore, it is important to get familiarized with its structure shown below.

| <code>indexList</code> | <code>totalStart</code> | <code>totalEnd</code> | <code>bosonStart</code> | <code>bosonEnd</code> | <code>spinIndex</code> | <code>total photon</code> | <code>total spin</code> |
|------------------------|-------------------------|-----------------------|-------------------------|-----------------------|------------------------|---------------------------|-------------------------|
| sector 1               |                         |                       |                         |                       | $\vdots$               |                           |                         |
| $\vdots$               |                         |                       |                         |                       | $\vdots$               |                           |                         |
| sector $\ell$          | $(\ell,1)$              | $(\ell,2)$            | $(\ell,3)$              | $(\ell,4)$            | $(\ell,5)$             | $(\ell,6)$                | $(\ell,7)$              |
| $\vdots$               |                         |                       |                         | $\vdots$              |                        |                           |                         |

- Col 1: Start index within the total basis set used in the `psiInitial` variable
- Col 2: End index within the total basis set
- Col 3: Start index within the boson basis set
- Col 4: End index within the boson basis set
- Col 5: Spin index
- Col 6: Photon excitation number
- Col 7: Spin excitation number

```
indexList = [];
lastIndexBoson = 0;
lastIndexTotal = 0;
```

We first find the indices of the spin basis with the correct number of up spins. Then, for each of the spins found, we create the indices described above and store them in `indexList`.

```
for ii=m:-1:m_min
    spinBasisIndices = find(sum(spinBasis,2) == m-ii);
    photonPartSize = nchoosek(L+ii-1,ii);
    for jj=1:length(spinBasisIndices)
        indexList = [indexList;...
            lastIndexTotal+1 lastIndexTotal+photonPartSize ...
            lastIndexBoson+1 lastIndexBoson+photonPartSize ...
            spinBasisIndices(jj) ii sum(spinBasis(spinBasisIndices(jj),:))];
        lastIndexTotal = lastIndexTotal + photonPartSize;
    end
    lastIndexBoson = lastIndexBoson + photonPartSize;
end
```

Note that we have not created the total basis set, but merely the indices of different sectors of the total basis set. When we create the initial condition for our setup via `generatePsi.m`, these indices will be utilized heavily.

```
end
```



## createPhotonBasis.m Create Photon Basis

This routine creates a bosonic basis for a lattice of length  $L$  where  $m$  photons exist. The basis is in the occupation number representation. This code is based on the algorithm explained in the following paper.

Zhang, J. M. & Dong, R. X,  
 “Exact diagonalization: the Bose-Hubbard model as an example”  
*European Journal of Physics*, 2010, 31, 591.  
<http://stacks.iop.org/0143-0807/31/i=3/a=016>

```
function out = createPhotonBasis(m,L)
```

Total number of ways of distributing  $m$  balls in  $L$  urns is given by  $\binom{L+m-1}{m}$ . The variable `out` stores the basis vectors.

```
len = nchoosek(L+m-1,m);  
out = zeros(len,L);
```

The following algorithm is from section three of the paper cited above. Initial state is the highest one  $|m, 0, 0, \dots, 0\rangle$ .

```
dum = zeros(1,L);  
nextdum = zeros(1,L);  
dum(1) = m;  
out(1,:) = dum;  
  
for ii=2:len  
    k = findK(dum);  
    if(dum(k)<=0)  
        error('Debug the code!');  
    end  
    if(k>1)  
        for jj=1:(k-1)  
            nextdum(jj) = dum(jj);  
        end  
    end  
    nextdum(k) = dum(k)-1;  
    nextdum(k+1) = m - sum(nextdum(1:k));  
    dum = nextdum;  
    nextdum = zeros(1,L);  
    out(ii,:) = dum;  
end
```

Sort the output so that the lowest state is the first.

```
out = out(len:-1:1,:);  
end
```

This is an auxiliary function used in the algorithm.

```
function k=findK(in)  
L = length(in);  
for ii=1:L-1  
    if(in(ii)~=0)  
        if(ii==L-1)  
            k=L-1;  
            break;  
        elseif(sum(in(ii+1:L-1))==0)  
            k=ii;  
            break;  
        end  
    end  
end  
end  
end
```

## createSpinBasis.m Create Spin Basis

This routine creates spin basis for  $n$  spins. The basis is in the occupation number representation, i.e.,  $|\uparrow_1\downarrow_2\cdots\uparrow_n\rangle$ .

```
function out = createSpinBasis(n)
```

There will be  $2^n$  states for  $n$  spin  $\frac{1}{2}$  qubits.

```
len = 2^n;
```

The algorithm for creating the states is quite simple. We will create the binary representation of the the numbers  $0 \dots 2^n - 1$  where the presence of bit 1 will refer to spin up,  $|\uparrow\rangle$ , and the presence of bit 0 will signal spin down,  $|\downarrow\rangle$ . We make use of the function `de2bi` for this purpose. Note that the most significant digit is at the leftmost side.

```
out = de2bi(0:len-1,'left-msb');
```

## generatePsi.m Generate the Initial State

This function will initialize the multi photon wavepacket in the occupation state basis. The initialization will be made in terms of the Kronecker product of single photon wavefunctions (properly symmetrized) with different qubit states. Each single photon wavefunction is specified by its wavepacket as a function of spatial coordinates via the use of function handles.

```
function generatePsi(initialStateParams)
```

The initial state of the wavepacket is described in a struct array, `initialStateParams`, consisting of the fields `qubitStates`, `photonStates`, `weights`. For instance, to be able to set the initial state to

$$|\Psi\rangle = A_1|m_1\rangle_{p_1} \otimes |\downarrow_1\downarrow_2\uparrow_3\rangle_s + A_2|m_2\rangle_{p_2} \otimes |\downarrow_1\uparrow_2\downarrow_3\rangle_s + A_3|m_3\rangle_{p_3} \otimes |\uparrow_1\downarrow_2\downarrow_3\rangle_s$$

where  $|m_1\rangle_{p_1}$  is a normalized, symmetrized photon state with  $m_1$  photons and  $A_1$  is the relevant complex amplitude, one should set `qubitStates` as  $\{[0\ 0\ 1], [0\ 1\ 0], [1\ 0\ 0]\}$  by mapping down-spins to 0 and up-spins to 1. Incidentally, these states refer to the 2nd, 3rd and 5th rows of the `createSpinBasis(3)` command. The spin order is from left to right. `weights` are simply given as  $\{A_1, A_2, A_3\}$  subject to the constraint  $\sum_n |A_n|^2 = 1$ . In order to describe the wave packet  $|m_1\rangle_{p_1}$  one should specify the function handles for  $m_1$  photons in a cell array.

The definition of a symmetrized  $m$ -photon wavefunction in a lattice of  $L$  points is given by<sup>1</sup>

$$|n_1 n_2 \dots n_L\rangle = \frac{1}{\sqrt{m! \prod_{\alpha} n_{\alpha}!}} \sum_P |\psi\rangle_{P_1} |\psi\rangle_{P_2} \dots |\psi\rangle_{P_m}$$

where  $n_{\alpha}$  denotes the number of photons in position  $\alpha \in [1..L]$ ,  $P$  stands for all permutations of the  $m$  single photon states  $|\psi\rangle$  described by the function handles.

The output, that is the initial state, will be put in the global variable `psiInitial`. Before this functions is called, `createFullBasis` should be invoked to create the global variables `indexList`, `bosonBasis` and `spinBasis`.

```
global indexList;
global bosonBasis;
global spinBasis;
global psiInitial;
```

Initialize `psiInitial` to the size of the basis. See `createFullBasis` documentation for a description of `indexList` data structure.

```
psiInitial = zeros(indexList(end,2),1);
```

Check to make sure the weights are subject to the constraint  $\sum_n |A_n|^2 = 1$ .

```
if sum(abs([initialStateParams.weights]).^2)-1 > 5*eps
    error('Weights are not normalized. Exiting.');
```

```
end
```

Check to make sure that each qubit state is unique. For instance,  $\{[0\ 0\ 1], [0\ 1\ 0], [1\ 0\ 0], [0\ 1\ 0]\}$  would not be allowed.

```
qubitStateArray = reshape([initialStateParams.qubitStates],length(spinBasis(1,:)),[]);
[CC,ia,ic]=unique(qubitStateArray,'rows');
if length(ia)~= length(initialStateParams)
    error('Duplicate qubit states. Exiting.');
```

```
end
```

We will now go through all the states defined in `initialStateParams` and update the relevant parts of `psiInitial`.

```
for kk=1:length(initialStateParams)
    m = length(initialStateParams(kk).photonStates); % number of photons
    L = size(bosonBasis,2); % lattice size
    storage = zeros(m,L); % used to store single photon states
    x = 1:L; % space variable
    qubit = initialStateParams(kk).qubitStates;
```

<sup>1</sup>See Negele, J. W., Orland, H. (1988). Quantum many-particle systems. Redwood City, Calif: Addison-Wesley Pub. Co. pp. 4–8. <http://www.worldcat.org/oclc/16404526>

```

% find the qubit sector number within the spinBasis
% sector number is obtained from the sorting of spins in indexList
[tf,spinIndex]=ismember(qubit,spinBasis,'rows');
if tf == 0 error('Spin not found. Exiting.');
```

```

end
sector = find(indexList(:,5) == spinIndex);
if isempty(sector) error('Sector not found. Exiting.');
```

```

end
totalStart = indexList(sector,1);
totalEnd = indexList(sector,2);
bosonStart = indexList(sector,3);
bosonEnd = indexList(sector,4);
if m ~= indexList(sector,6) error('Photon number mismatch. Exiting.');
```

```

end

% populate the storage with single photon normalized wavefunctions
for ii = 1:m

    % get the function handler
    fhandle = initialStateParams(kk).photonStates{1,ii};

    % set the storage photons
    storage(ii,:) = fhandle(x);

end

bosonIndices = bosonStart:bosonEnd;
totalIndices = totalStart:totalEnd;
if length(bosonIndices) ~= length(totalIndices)
    error('indexList total/boson indices corrupted. Exiting.');
```

```

end

% Create symmetric permutations of the m-photons and express them in the
% number state basis
symmetricSum = perms(1:m); % all permutations of m photons
for ii=1:length(bosonIndices)
    basis = bosonBasis(bosonIndices(ii),:);
    indices = find(basis); % locations of photons
    coords = []; % Photon coordinates
    % Find the coordinates of m photons
    for jj=1:length(indices)
        coords = [coords repmat(indices(jj),1,basis(indices(jj)))];
    end

    % Multiply and add all symmetric combinations of photons
    if m>0
        for jj=1:size(symmetricSum,1)
            linearIndices = sub2ind(size(storage),symmetricSum(jj,:),coords);
            psiInitial(totalIndices(ii)) = ...
                psiInitial(totalIndices(ii)) + prod(storage(linearIndices));
        end
    else
        % If there are no photons, there is only one state:
        % atom is excited
        psiInitial(totalIndices(ii)) = 1;
    end
    % Apply the normalization factor
    psiInitial(totalIndices(ii)) = ...
        psiInitial(totalIndices(ii))/(sqrt(factorial(m)*prod(factorial(basis(indices)))));

end

% Normalize the resulting wavefunction in case the one-photon wavepackets

```

```

% are not orthogonal. Each sector should be normalized within itself.
% When the photon states in the storage variable are
% orthogonal, the sector, at this stage, has a total normalization of 1/N!(N=photon number)
% which should be fixed. On the other extreme, when the photon states
% are identical, the total normalization turns out to be exactly 1. When the
% photon states are not orthogonal, the value will be in between the
% two extremes. The reason for this behavior is that normalization in
% the occupation basis set only counts distinct terms and hence
% introduces a 1/N! factor in front of the
% integration in the real-space symmetric wavefunction.

% Normalize the sector within itself
psiInitial(totalIndices) = psiInitial(totalIndices) ./ ...
    norm(psiInitial(totalIndices));

% Apply the weight factor
psiInitial(totalIndices) = psiInitial(totalIndices) .* ...
    initialStateParams(kk).weights;
end
% Check the normalization of the final wavefunction and issue an error
% message if it is not 1.
if abs(norm(psiInitial) - 1) > 3*eps
    error('psiInitial norm = %20.20g should have been 1.',norm(psiInitial));
end
% Fix normalization to filter out numerical noise.
psiInitial = psiInitial / norm(psiInitial);

end

```

## generateH.m Generate the Hamiltonian

This function will generate the Hamiltonian,  $H$ , in the number state representation basis. The Hamiltonian is given as

$$H = \underbrace{-J \sum_{i=1}^{L-1} (a_{i+1}^\dagger a_i + a_i^\dagger a_{i+1})}_{\text{Hopping}} + \underbrace{\sum_{s=1}^n \frac{\Omega_s}{2} \sigma_{z_s}}_{\text{Sigma}} + \underbrace{\sum_{s=1}^n V_s (\sigma_s^+ a_{x_s} + a_{x_s}^\dagger \sigma_s^-)}_{\text{Coupling}}$$

where  $L$  is the size of the lattice,  $n$  is the number of qubits,  $x_s$  are the locations of the qubits,  $J$  is the hopping parameter,  $\Omega_s$  are the energy separations between the ground and excited states of the qubits,  $V_s$  are the coupling parameters,  $a_i$  is the annihilation operator for photons at lattice site  $i$ ,  $\sigma^-$  is the qubit lowering operator. An example visualization of the 1D lattice for  $L = 11$  and  $n = 3$  is given below. Qubits are ordered from left to right.

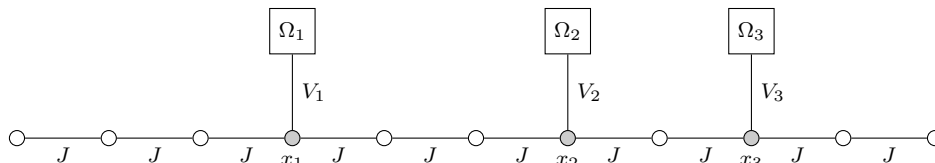

In the following, we will implement each part of  $H$  above for every sector in the basis. We will need to figure out the locations of a variety of basis vectors and to that end will use the auxiliary function `getIndex`.

```
function H = generateH(J,Oms,Vs,xs)
```

`Oms` stands for  $\Omega_s$ , `Vs` for  $V_s$ , `xs` for  $x_s$  i.e. they are vectors with  $n$  elements holding qubit parameters. `J` is the tight binding coupling parameter  $J$ .

```
global indexList;
global bosonBasis;
global spinBasis;
```

The dimension of  $H$  is  $\text{dim} \times \text{dim}$ . See `createFullBasis` documentation for a description of `indexList` data structure.

```
dim = indexList(end,2); % total size
L = size(bosonBasis,2); % lattice length
```

These variables hold the sparse matrix definition vectors for the hopping and coupling parts of the Hamiltonian. Each sector in the total basis has a number of photons. The maximum non-zero elements in the hopping part of the Hamiltonian is given by the relevant size of the sector multiplied by the number of photons in that sector, added up for all the sectors. Similarly, for the coupling part, one calculates  $\binom{L+m-2}{m-1} \times (\# \text{ of down spins})$ —where  $m$  is the number of photons for each sector—and adds them up since we are interested in those states that have a photon at the qubit location and the qubit in the down state.

```
hoppingSize = 0;
coupleSize = 0;
for mm=1:size(indexList,1)
    hoppingSize = hoppingSize + (indexList(mm,2)-indexList(mm,1)+1)*indexList(mm,6);
    if indexList(mm,6) > 0
        coupleSize = coupleSize + nchoosek(L+indexList(mm,6)-2,indexList(mm,6)-1)*...
            length(find(spinBasis(indexList(mm,5)) == 0 ));
    end
end

iListHop = ones(1, hoppingSize);
jListHop = ones(1, hoppingSize);
sListHop = zeros(1, hoppingSize);
listIndexHop = 1;
iListCouple = ones(1, coupleSize);
jListCouple = ones(1, coupleSize);
sListCouple = zeros(1, coupleSize);
listIndexCouple = 1;
```

```

sector = 1;
for jj=1:dim
    if jj > indexList(sector,2)
        sector = sector+1;
    end
    basis_p = bosonBasis(jj-indexList(sector,1)+indexList(sector,3),:);
    basis_s = spinBasis(indexList(sector,5),:);
    % Create Hhop by going through  $\sum_1^{L-1} a^{\dagger}_{k+1} a_k$ 
    % then add the hermition conjugate that is  $a^{\dagger}_k a_{k+1}$ 
    indices = find(basis_p(1:L-1));
    for kk=indices
        % Create the basis with one boson moved from site k to k+1
        hopBasis = basis_p;
        hopBasis(kk) = hopBasis(kk)-1;
        hopBasis(kk+1) = hopBasis(kk+1)+1;
        % Find the index of the hopBasis
        ii = getIndex(hopBasis,basis_s);
        % Record the locations and matrix value
        iListHop(listIndexHop) = ii;
        jListHop(listIndexHop) = jj;
        sListHop(listIndexHop) = sqrt(basis_p(kk))*sqrt(basis_p(kk+1)+1);
        listIndexHop = listIndexHop + 1;
    end
    % Create the coupling part of the Hamiltonian
    for kk=1:length(xs)
        x0=xs(kk);
        if(basis_p(x0) > 0 && basis_s(kk) == 0)
            % Create the basis with one boson removed from site x0 and
            % qubit at x0 in the up state
            coupleBasis = basis_p;
            coupleBasis(x0) = coupleBasis(x0)-1;
            coupleSpin = basis_s;
            coupleSpin(kk) = 1;
            ii = getIndex(coupleBasis,coupleSpin);
            % Record the locations and matrix value
            iListCouple(listIndexCouple) = ii;
            jListCouple(listIndexCouple) = jj;
            sListCouple(listIndexCouple) = Vs(kk)*sqrt(basis_p(x0));
            listIndexCouple = listIndexCouple + 1;
        end
    end
end
% add the conjugate transpose as well when building H
Hhop = sparse(iListHop,jListHop,sListHop,dim,dim);
Hcouple = sparse(iListCouple,jListCouple,sListCouple,dim,dim);

% Create the sigma part
iList = 1:dim;
jList = 1:dim;
sList = zeros(1,dim);
%  $(-1)^{\dots}$  part simply maps down qubits denoted by 0 to -1, and up qubits
% denoted by 1 to 1.
for kk=1:size(indexList,1)
    sList(indexList(kk,1):indexList(kk,2)) = ...
        0.5 * sum((-1).^(spinBasis(indexList(kk,5),:)+1) .* 0ms);
end
Hsigma = sparse(iList,jList,sList,dim,dim);
% Build the full Hamiltonian
H = -J*(Hhop + Hhop') + Hsigma + (Hcouple + Hcouple');

```

## getIndex.m Get the Index for an Arbitrary State

This function returns the index value of an arbitrary state where  $m$  bosons are distributed in a lattice of length  $L$  with  $n$  qubits. Algorithm is from the following paper.

Liang, S.  
 “A perfect hashing function for exact diagonalization of many-body systems of identical particles”  
*Computer Physics Communications*, 1995, 92, pp. 11–15  
<http://www.sciencedirect.com/science/article/pii/001046559500108R>

```
function index = getIndex(x,s)

global indexList;

x is the boson part, s is the spin part. We need access to the global variable indexList created in createFullBasis.m
script.

L = length(x);
% get the total number of excitations in the bosonic part
m = sum(x);
% and also in the spin part
n = sum(s);

% stores location of each photon 0 <= p1 <= p2 <= ... < L
plist = zeros(m,1);

% find the nonzero indices
nonzeroIndices = find(x);

for ii=1:length(nonzeroIndices)
    k = nonzeroIndices(ii);
    nphoton = x(k);
    k = L-k; % map the index to (L-1) .. 0
    for jj=1:nphoton
        plist(m) = k;
        m = m-1;
    end
end

index = 0;
for ii=1:length(plist)
    if(plist(ii)+ii-1 >= ii)
        index = index + nchoosek(plist(ii)+ii-1,ii);
    end
end

The code above gives a number between  $0 \dots (L-1)$  stored in index. Add 1 to get 1 based indexing.

indexBoson = index+1;

To get the spin index part calculate the decimal equivalent of the spin and add one.

indexSpin = bi2de(s,'left-msb') +1;

Get the starting index for the spin part and add indexBoson-1 to get the final result.

index = indexList(find(indexList(:,5) == indexSpin,1),1) + indexBoson -1;

end
```



## getExpectation.m Get Various Expectation Values and Measurements

This function will calculate the expectation values of a number of operators,  $\hat{O}$ , for a given state of the wavefunction,  $|\Psi\rangle$ . That is, it will output  $\langle\Psi|\hat{O}|\Psi\rangle$ . At the moment, the calculated expectation values are for

$$n_x \equiv \langle\Psi|a_x^\dagger a_x|\Psi\rangle \quad n_s \equiv \langle\Psi|\sigma_s^+ \sigma_s^-|\Psi\rangle \quad R \equiv \sum_{i=1}^{x_1-1} n_i + \frac{1}{2}n_{x_1} \quad T \equiv \sum_{i=x_n+1}^L n_i + \frac{1}{2}n_{x_n}$$

where  $n_x$  is the expected value of photons at position  $x$ ,  $n_s$  is the probability of having qubit  $s$  in the up state,  $x_1$  is the position of the first qubit,  $x_n$  that of the last qubit.

`varargout` is used to optionally output the expected number of photons as function of lattice position *and* sector number.

```
function [nx,ns,R,T,varargout]=getExpectation(xs)
% xs are the qubit locations in the lattice
global indexList;
global bosonBasis;
global spinBasis;
global psi;
% initialization
L = size(bosonBasis,2); % Lattice size
n = size(spinBasis,2); % Number of qubits
dim = length(psi); % total size of the basis
nx = zeros(1,L);
ns = zeros(1,n);
R = 0;
T = 0;
% size(indexList,1) gives the number of sectors
if(nargout==5)
    nxSectors = zeros(size(indexList,1),L);
end

% Calculate nx
sector = 1;
for jj=1:dim
    if jj > indexList(sector,2)
        sector = sector+1;
    end
    basis_p = bosonBasis(jj-indexList(sector,1)+indexList(sector,3),:);
    indices = find(basis_p);
    nx(indices) = nx(indices) + abs(psi(jj))^2 * basis_p(indices);
    if(nargout==5)
        nxSectors(sector,indices) = nxSectors(sector,indices) + ...
            abs(psi(jj))^2 * basis_p(indices);
    end
end

% Calculate ns
for kk=1:size(indexList,1)
    basis_s = spinBasis(indexList(kk,5),:);
    indices = find(basis_s);
    ns(indices) = ns(indices) + sum(abs(psi(indexList(kk,1):indexList(kk,2))).^2);
end

% Calculate R and T
R = sum(nx(1:xs(1)-1)) + 0.5 * nx(xs(1));
T = sum(nx(xs(end)+1:end)) + 0.5 * nx(xs(end));
% Output optional sector based nxSectors
if nargout==5
    varargout{1} = nxSectors;
end
end
```
